# Supplementary material for: What's in the laundromat? Mapping and characterising offshore owned domestic property in London
Source: arXiv:2207.10931 ancillary file (2022-07-22)
Supplement: Supplementary file 1 [file Offshore_London_Supplementary_Material.pdf]

# Inspecting the laundromat: Supplementary Material

anonymous

June 2022

## 1 Introduction

This document includes contains the supplementary material for the paper 'Inspecting the laundromat: Mapping and characterising offshore owned domestic property in London'. It covers supporting information that is not key to understanding the main paper but provides additional details and nuance to the main method and analysis

## 2 Description of the enhanced OCOD dataset

The enhanced OCOD dataset is made up of 19 data columns. These data columns are defined below

| | Name | Type | Description |
|---|---|---|---|
| 1 | title_number | string | The unique id provided by the land registry |
| 2 | nested_title | logical | Is the property part of a nested title? The original OCOD dataset also has 'multiproperty' this similar but the other properties are not included in that dataset. The Land registry appears to be replacing that column with the nested approach. There are only about 800 of 'multiproperties' so were not considered as part of the pipeline |
| 3 | nested_id | integer | A value identifying the property within the a nested title number |
| 4 | unique_id | string | The title number and nested id separated by a hyphen |
| 5 | unit_id | string | The id of the flat, unit, carparking space etc. Usually a number but can have other formats |
| 6 | unit_type | string | The type of unit, e.g. flat. |
| 7 | building_name | string | The name of the building associated with the title number |
| 8 | street_number | string | The positional reference on the street for the title number. Usually a number, but can have other formats. |
| 9 | street_name | string | The street name |
| 10 | postcode | string | Property postcode |
| 11 | city | string | The City, town village or area of the property |
| 12 | property_address | string | The full property address as provided in the original OCOD dataset |
| 13 | district | string | The district name as provided in the original OCOD dataset. This is not the name standard used by the ONS |
| 14 | region | string | Represents the broad area of England and Wales that the property is in. |
| 15 | lsoa11cd | string | LSOA census geography code for census 2011 |
| 16 | msoa11cd | string | MSOA census geography code for census 2011 |
| 17 | lad11cd | string | Local Authority district census geography code for census 2011. Generally maps to the 'district' category. |
| 18 | class | string | The property classification using the Type 1 classification method |
| 19 | class2 | string | The property classification using the Type 1 classification method. This method is generally a better choice as it has high performance but much lower 'unknowns' |

## 3 Training details

The configuration files for the spaCy models used to create the pipeline can be found in the github repo. Although in the paper we refer to the RoBERTa transformer architecture, we found very little improvement over the original denoised dataset. However, using the spaCy model is a convenient way of labelling the original OCOD dataset. To avoid issues with GPU requirements and long labelling times we switched the RoBERTa model for a simple vector representation of words. This allowed a CPU optimised model to be trained. This is the model that is currently available for the pipeline. It's performance is essentially identical to the RoBERTa model. The spaCy model is available from an open dropbox folder at `https://www.dropbox.com/sh/kom162tjwgo7c2h/AABWOygE8gtJhgIKhFYtCvWha?dl=0`, it is compressed using tar.xz format. Other formats can be made available upon request. In order to reproduce the pipeline exactly the correct data files are required. However, generally it is advisable to use the most upto date version available of the necessary files. For example and out of date ONSPD database may mean that new postcodes are not recognised missing out on matching groups of properties.

| Dataset | Original dates names |
|---|---|
| OCOD dataset | OCOD_FULL_2022_02 |
| ONSPD | ONSPD_NOV_2021_UK |
| Price Paid dataset | years 2017-2021 |
| VOA ratings list | uk-englandwales-ndr-2017-listentries-compiled-epoch-0029-baseline-csv |

## 4 Incorporation country details

Below are two plots providing more details on the country of incorporation of offshore owned domestic properties in London. Figure 1 shows the counts of properties or title deeds by country of incorporation. There is a clear difference between the data showed by the the Original OCOD dataset that was purely title numbers and the data showed by the Enhanced OCOD dataset which is the number of actual properties. The figure also shows that different territories tend to be used for different types of offshore, the BVI has very few nested properties whilst the British Crown Dependencies of Jersey, Guernsey and the Isle of Man, have a large amount. Figure 2 shows the relationship between the country of incorporation and Britain. As can be seen the Crown Dependencies (CD) account for a very large fraction of the total property, as do the British Overseas Territories (BOT), primarily due to the British Virgin Islands (BVI). In addition a significant fraction of the remaining property (11%) is owned by countries were British colonies but that became independent of Britain in the post World War 2 (PWWe) period.

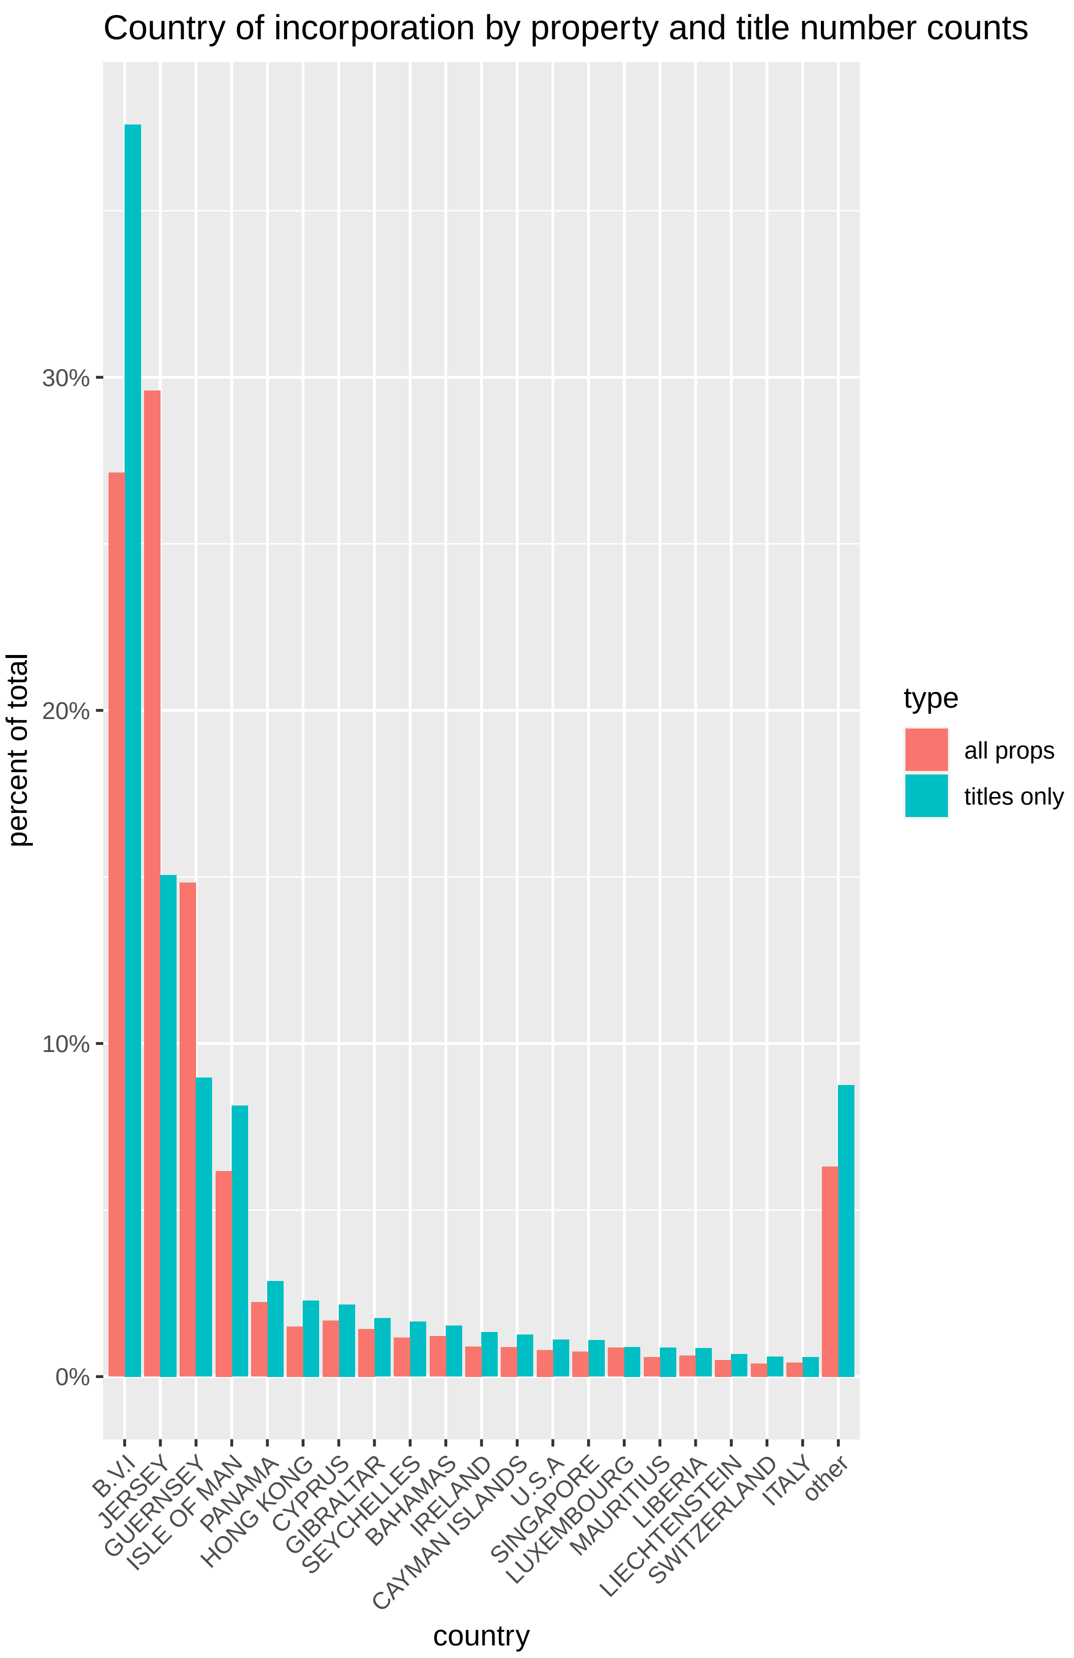


Figure 1: The figure shows the country of incorporation as a percent of total for both individual properties and individual title numbers. In both cases a small number of countries strongly associated with Britain a responsible for the majority.

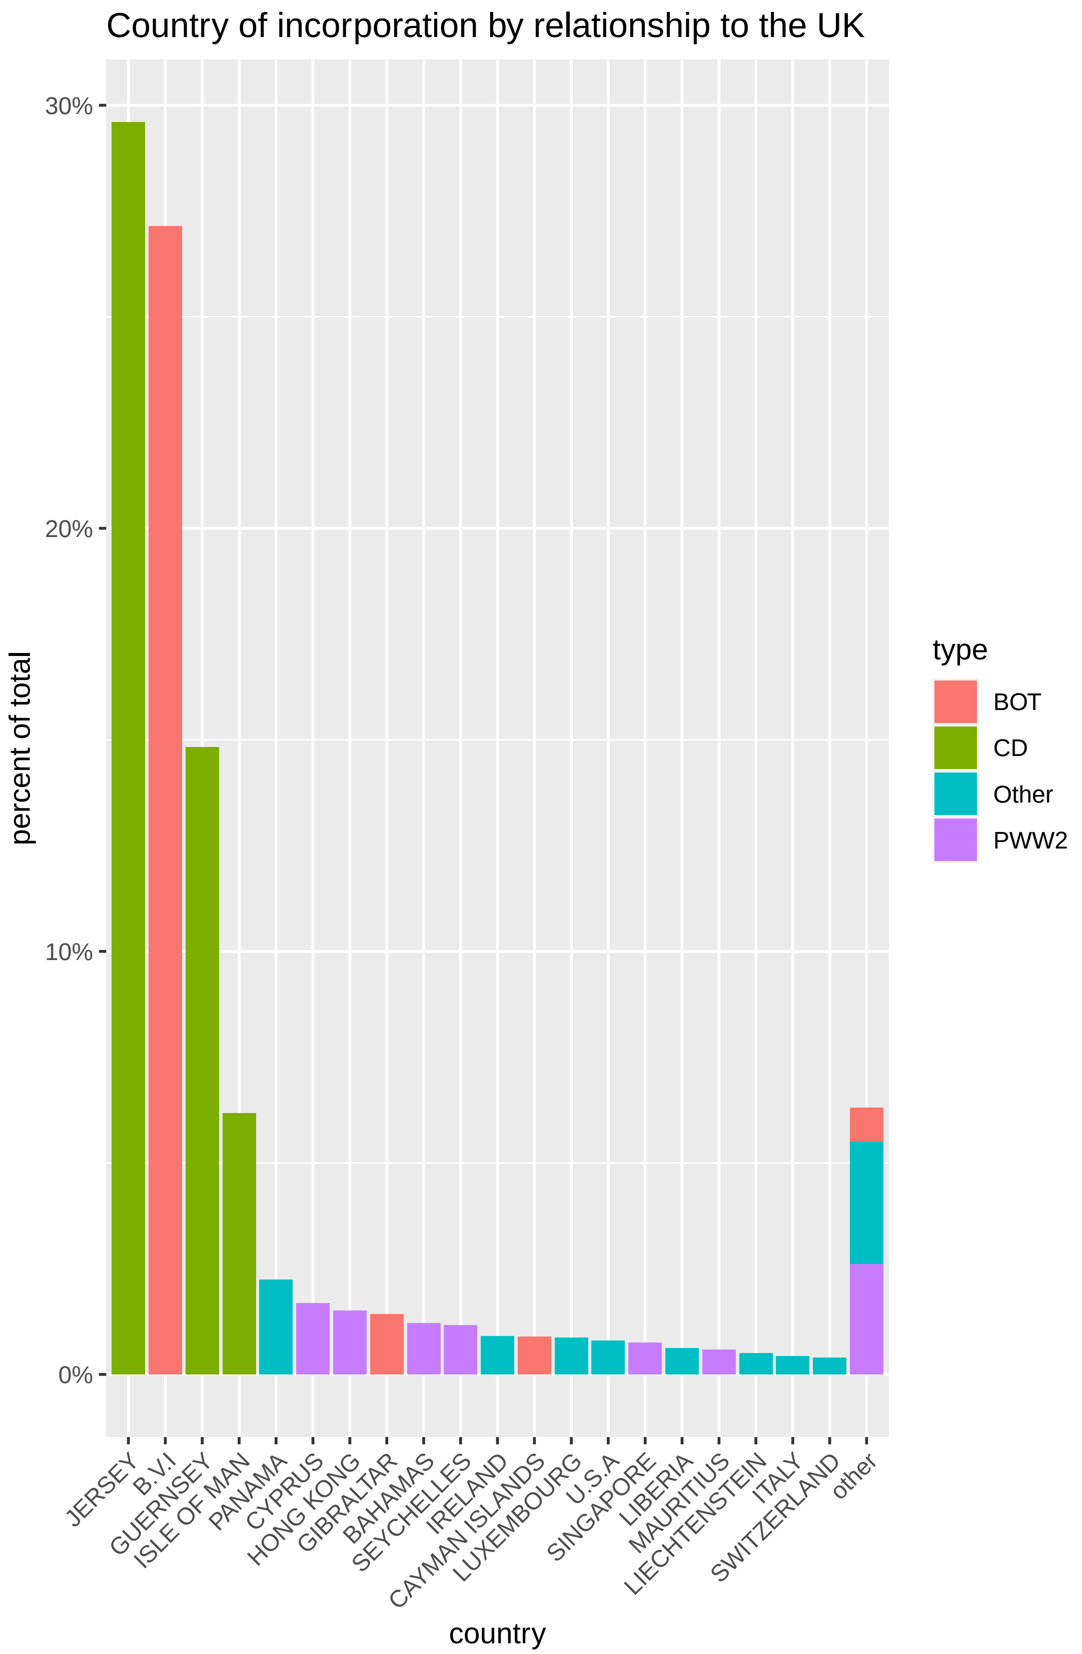


Figure 2: Figure shows the percent of properties by country of incorporation. Countries are coloured by their relationship to the UK. A large fraction of the properties belong to the Crown dependencies (CD), followed by British Overseas territories (BOT), In addition there are countries that gained independence from Britain Post World War 2 (PWW2)
